# Supplementary material for: Towards Perceiving Small Visual Details in Zero-shot Visual Question Answering with Multimodal LLMs
Source: arXiv:2310.16033 source file (2024-02-12)
Supplement: Supplementary file 2 [file question_types.tex]

\section{The Effect of Visual Cropping On Different Question Types.}
\input{sections/tab_question_types}

 % To gain deeper insight into the granular benefits of visual cropping, \cref{fig:question_type} shows how the proposed visual cropping methods impact the accuracy of zero-shot VQA models on various question types in VQAv2 (question types are explained in~\cref{tab:question_types} in Appendix). Questions concerning visual details, \ie, text reading and object attributes, gain the most from visual cropping, consistent with our findings in DTVQA and TextVQA. However, we observe that questions that require a global view of the image, \ie, localization and counting, become harder to answer as a result of visual cropping. This suggests that our mechanism for combining the original and cropped image tokens is not always successful in maintaining the global image information, encouraging future research on effectively combining image tokens.
